# Supplementary material for: Saliency-driven Word Alignment Interpretation for Neural Machine Translation
Source: arXiv:1906.10282 source file (2019-06-27)
Supplement: Supplementary file 1 [file appendix.tex]

\appendix
\section{Appendices}
\subsection{Stability Analysis}

We run de-en, en-fr, ro-en models multiple times to evaluate the variance of word alignment interpretation and its relationship with the choice of interpretation method.
Results are shown in Table~\ref{tab:res-stability}.
In general we find the variance of FConv and LSTM comparable, and that of Transformer is significantly higher.
Unfortunately, none of the word saliency methods explored here reduces the variance of interpretation.

\begin{table*}[t]
\centering
\scalebox{0.85}{
\begin{tabular}{@{}llll@{}}
\toprule
 & \textbf{de-en} & \textbf{en-fr} & \textbf{ro-en} \\ \midrule
\textbf{FConv} &  &  &  \\
Attention & 38.4 $\pm$ 0.374 & 23.2 $\pm$ 0.438 & 40.5 $\pm$ 0.178 \\
Smoothed Attention & 40.8 $\pm$ 0.268 & 23.8 $\pm$ 0.430 & 41.3 $\pm$ 0.249 \\
\cite{DBLP:conf/naacl/LiCHJ16} Grad & 38.9 $\pm$ 0.228 & 27.1 $\pm$ 0.367 & 41.9 $\pm$ 0.218 \\
\cite{DBLP:conf/naacl/LiCHJ16} SmoothGrad & 40.8 $\pm$ 0.130 & 27.1 $\pm$ 0.148 & 43.3 $\pm$ 0.311 \\
Ours Grad & 33.0 $\pm$ 0.327 & 24.9 $\pm$ 0.100 & 37.0 $\pm$ 0.122 \\
Ours SmoothGrad & 26.7 $\pm$ 0.296 & 20.9 $\pm$ 0.269 & 32.6 $\pm$ 0.218 \\
\textbf{LSTM} &  &  &  \\
Attention & 42.8 $\pm$ 0.112 & 32.3 $\pm$ 0.320 & 46.9 $\pm$ 0.277 \\
Smoothed Attention & 54.7 $\pm$ 1.76 & 34.9 $\pm$ 0.729 & 50.9 $\pm$ 0.430 \\
\cite{DBLP:conf/naacl/LiCHJ16} Grad & 41.1 $\pm$ 0.173 & 32.7 $\pm$ 0.381 & 44.6 $\pm$ 0.228 \\
\cite{DBLP:conf/naacl/LiCHJ16} SmoothGrad & 40.1 $\pm$ 0.415 & 32.9 $\pm$ 0.771 & 45.8 $\pm$ 0.456 \\
Ours Grad & 46.3 $\pm$ 0.918 & 41.1 $\pm$ 0.863 & 54.8 $\pm$ 1.10 \\
Ours SmoothGrad & 30.1 $\pm$ 0.549 & 26.2 $\pm$ 0.545 & 39.8 $\pm$ 0.274 \\
\textbf{Transformer} &  &  &  \\
Attention & 59.7 $\pm$ 2.12 & 45.6 $\pm$ 0.819 & 52.9 $\pm$ 0.776 \\
Smoothed Attention & 62.5 $\pm$ 2.12 & 43.6 $\pm$ 0.626 & 59.8 $\pm$ 1.22 \\
\cite{DBLP:conf/naacl/LiCHJ16} Grad & 52.4 $\pm$ 0.998 & 45.1 $\pm$ 1.22 & 46.7 $\pm$ 0.636 \\
\cite{DBLP:conf/naacl/LiCHJ16} SmoothGrad & 39.3 $\pm$ 2.30 & 27.6 $\pm$ 1.16 & 39.6 $\pm$ 1.44 \\
Ours Grad & 77.7 $\pm$ 0.524 & 70.4 $\pm$ 0.976 & 74.5 $\pm$ 1.33 \\
Ours SmoothGrad & 37.8 $\pm$ 1.09* & 28.7 $\pm$ 0.85 & 40.5 $\pm$ 1.05 \\ \bottomrule
\end{tabular}
}
\caption{Stability analysis of results with multiple runs in Table \ref{tab:main-res1}. Numbers affected by hyper-parameter tuning are marked with *.}
\label{tab:res-stability}
\end{table*}

\subsection{BLEU Score of the NMT System}
\begin{table}[h]
\scalebox{0.85}{
\begin{tabular}{@{}lllllll@{}}
\toprule
      & \textbf{de-en} & \textbf{en-de} & \textbf{en-fr} & \textbf{fr-en} & \textbf{ro-en} & \textbf{en-ro} \\ \midrule
fconv & 31.8           & 27.2           & 32.7           & 28.1           & 31.6           & 31.8           \\
LSTM  & 32.7           & 26.8           & 32.5           & 26.1           & 29.9           & 28.5           \\
TFM   & 36.6           & 31.1           & 34.9           & 33.9           & 33.8           & 34.9           \\ \bottomrule
\end{tabular}}
\caption{BLEU score of the NMT systems. For systems with multiple runs, the score shown here is the average.}
\label{tab:bleu}
\end{table}

\subsection{Extra SmoothGrad Figures}
\begin{figure*}[!btp]
    \hspace{-0.5cm}
    \includegraphics[scale=0.65]{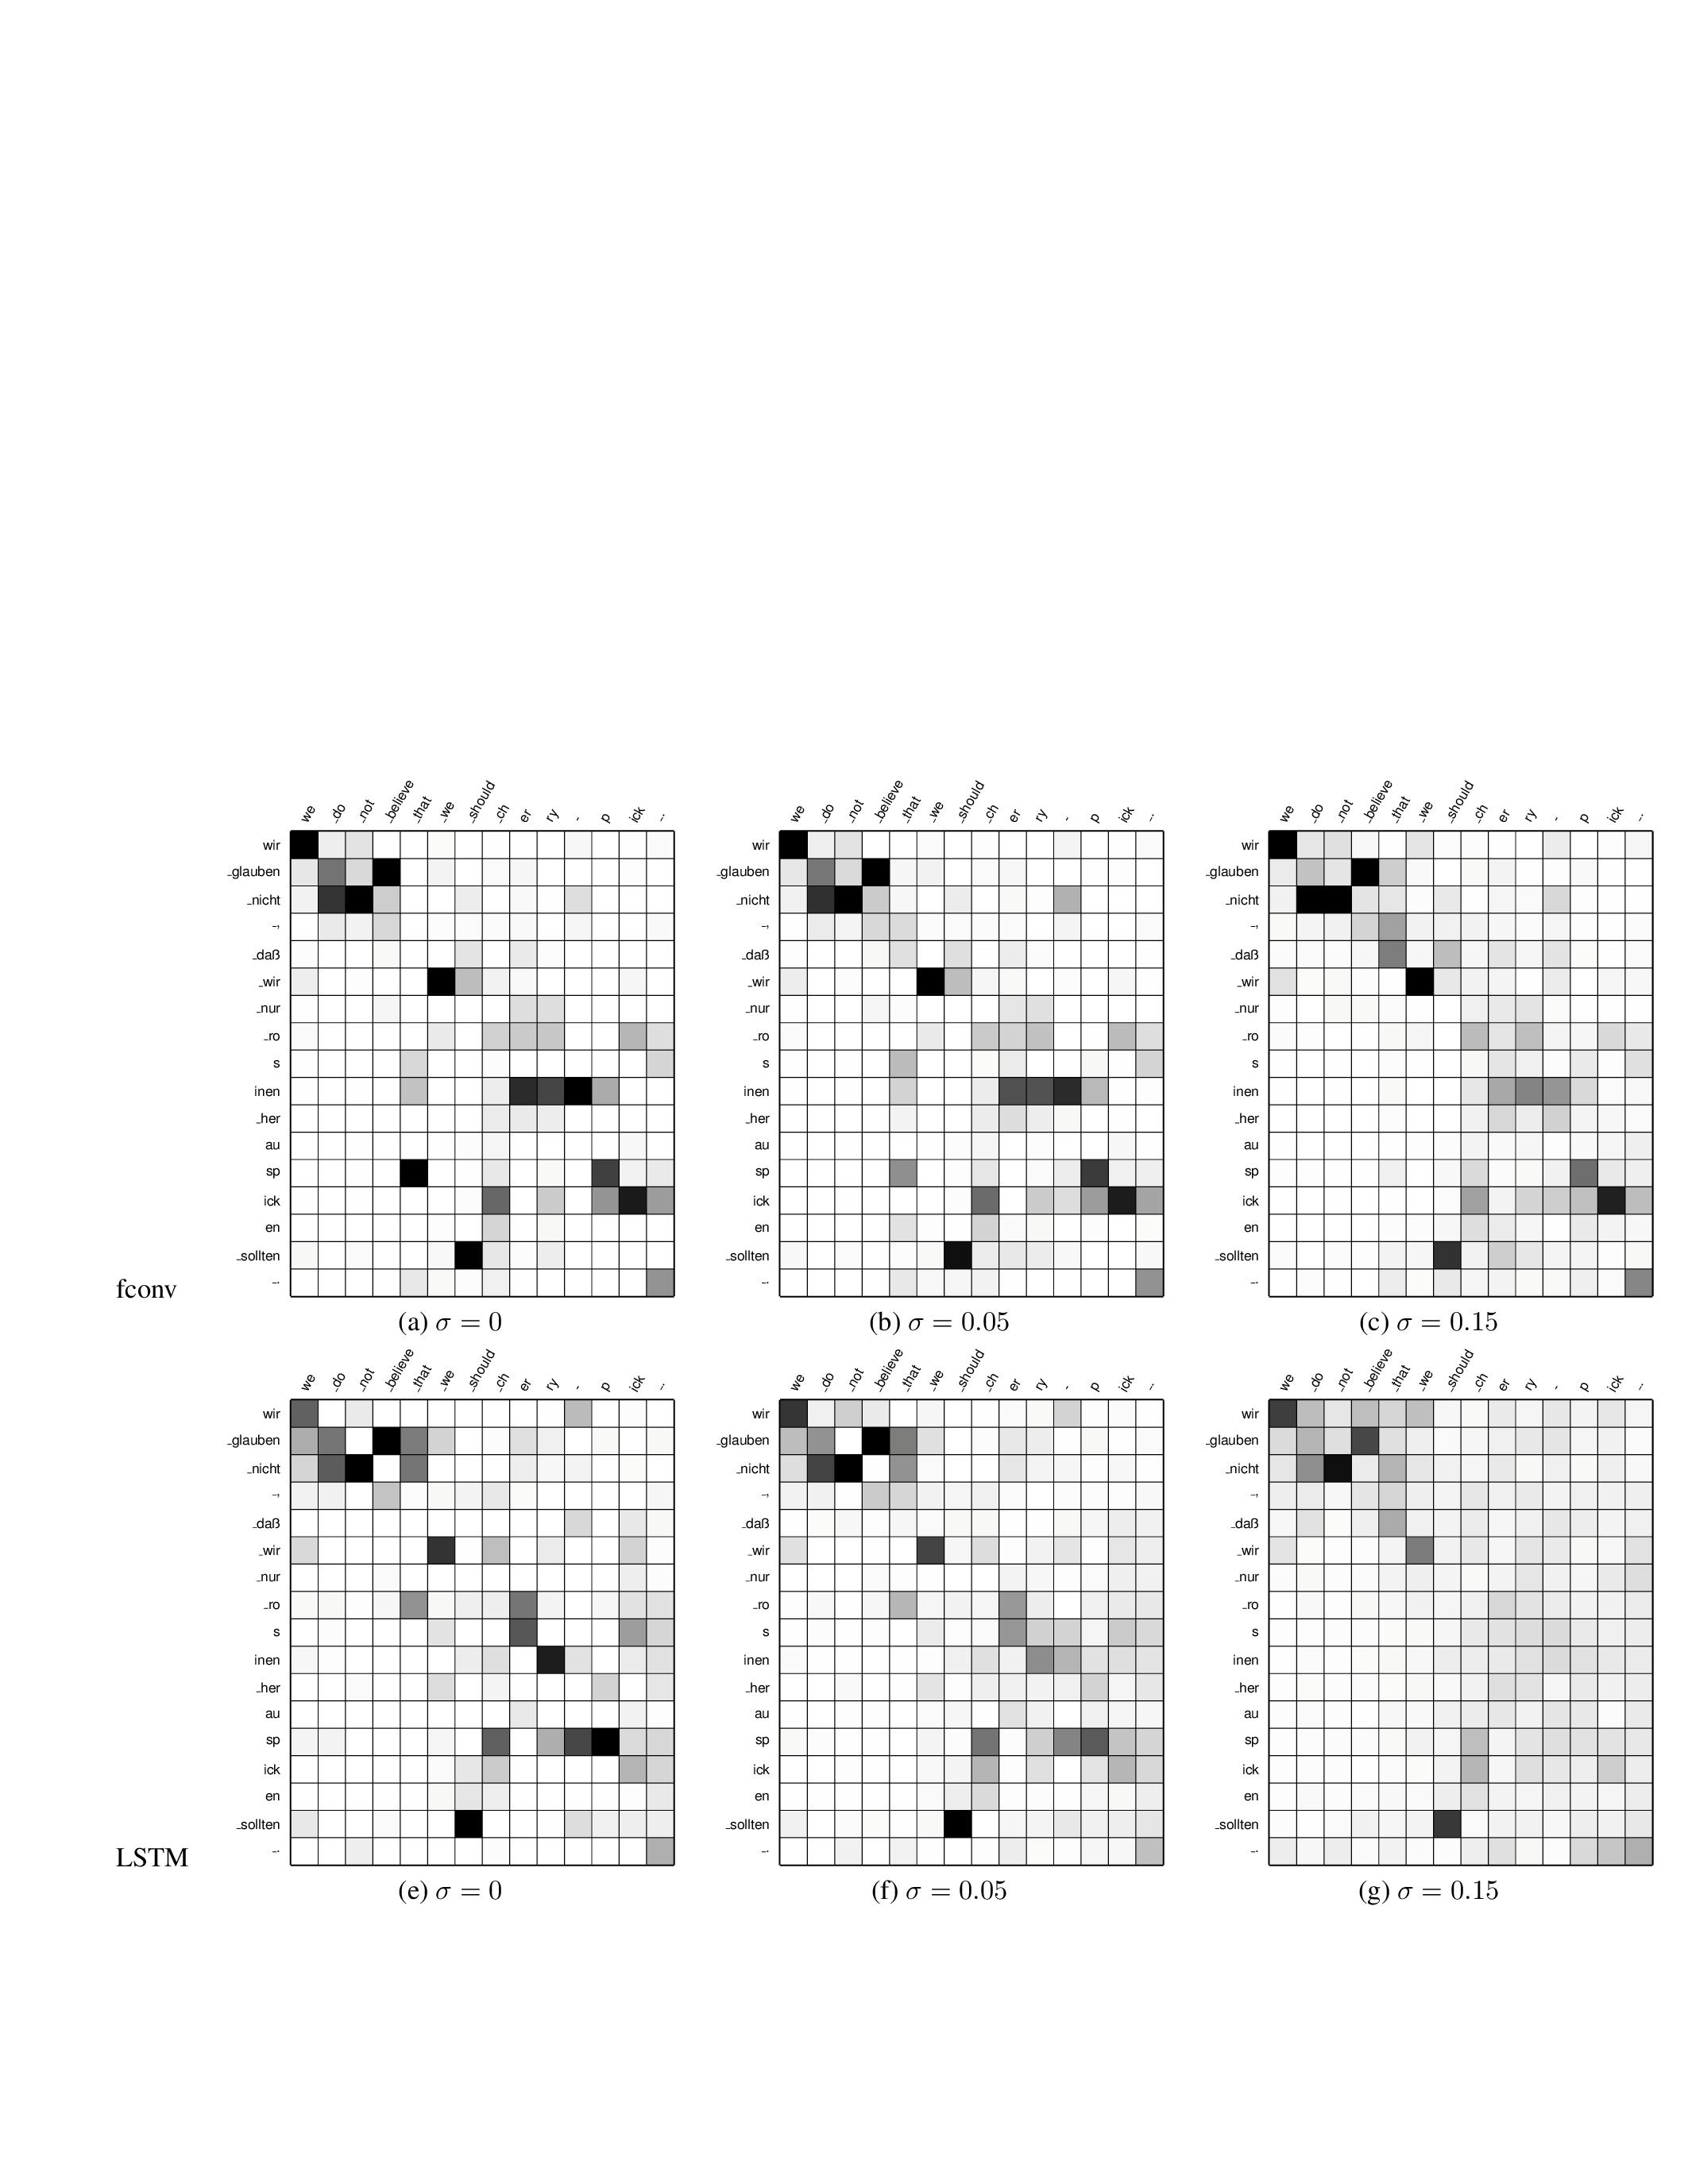}
    \caption{Salience interpretation of fconv and LSTM de-en model with different SmoothGrad noise values $\sigma$ ($n=30$).}
    \label{fig:extra_smoothgrad}
\end{figure*}
